# Supplementary material for: PIRLNav: Pretraining with Imitation and RL Finetuning for ObjectNav
Source: arXiv:2301.07302 source file (2023-03-26)
Supplement: Supplementary file 1 [file supplement.tex]

% % CVPR 2023 Paper Template
% % based on the CVPR template provided by Ming-Ming Cheng (https://github.com/MCG-NKU/CVPR_Template)
% % modified and extended by Stefan Roth (stefan.roth@NOSPAMtu-darmstadt.de)

% \documentclass[10pt,twocolumn,letterpaper]{article}

% %%%%%%%%% PAPER TYPE  - PLEASE UPDATE FOR FINAL VERSION
% \usepackage[review]{cvpr}      % To produce the REVIEW version
% %\usepackage{cvpr}              % To produce the CAMERA-READY version
% %\usepackage[pagenumbers]{cvpr} % To force page numbers, e.g. for an arXiv version

% \input{imports}
% % Include other packages here, before hyperref.
% \usepackage{graphicx}
% \usepackage{amsmath}
% \usepackage{amssymb}
% \usepackage{booktabs}
% \usepackage{tablefootnote}


% \newcolumntype{=}{% resets the row style
%   >{\gdef\@rowstyle{}}%
% }

% \newcolumntype{+}{% adds the current row style to the next column
%   >{\@rowstyle}%
% }

% % It is strongly recommended to use hyperref, especially for the review version.
% % hyperref with option pagebackref eases the reviewers' job.
% % Please disable hyperref *only* if you encounter grave issues, e.g. with the
% % file validation for the camera-ready version.
% %
% % If you comment hyperref and then uncomment it, you should delete
% % ReviewTempalte.aux before re-running LaTeX.
% % (Or just hit 'q' on the first LaTeX run, let it finish, and you
% %  should be clear).
% % \usepackage[pagebackref,breaklinks,colorlinks]{hyperref}

% % Support for easy cross-referencing
% \usepackage[capitalize]{cleveref}
% \crefname{section}{Sec.}{Secs.}
% \Crefname{section}{Section}{Sections}
% \Crefname{table}{Table}{Tables}
% \crefname{table}{Tab.}{Tabs.}


% %%%%%%%%% PAPER ID  - PLEASE UPDATE
% \def\cvprPaperID{3969} % *** Enter the CVPR Paper ID here
% \def\confName{CVPR}
% \def\confYear{2023}


% \begin{document}

% %%%%%%%%% TITLE - PLEASE UPDATE
% % \title{Effectiveness of Human Demonstrations for RL Finetuning}
% % \title{Human demonstrations in \objnav: how to best combine imitation and reinforcement learning?}
% % \title{Not all demonstrations are created equal: an \objnav case study for effectively combining imitation and reinforcement learning}
% % \title{Scaling laws of imitation $\rightarrow$ reinforcement learning in \objnav}
% \title{Supplement - PIRLNav: Pretraining with Imitation and RL Finetuning for \objnav}

% \author{}

% % \maketitle


% %%%%%%%%% ABSTRACT
% \input{sections/appendix/appendix}

% %%%%%%%%% REFERENCES
% \bibliographystyle{ieeetr}
% \bibliography{strings,main}


% \end{document}
